# Supplementary material for: ConEx: Efficient Exploration of Big-Data System Configurations for Better Performance
Source: arXiv:1910.09644 source file (2020-06-22)
Supplement: Supplementary file 1 [file 11_response_major_revision.tex]

\pagebreak
\newpage
\pagenumbering{Roman}
\renewcommand{\baselinestretch}{0.75}
\renewcommand*{\thesection}{\Alph{section}}
\nobalance
\section*{RESPONSE TO REVIEWERS}
\bigskip
\section*{Editor}

\noindent{\em The reviewers have a lot of positive responses about the manuscript. However, there are some major concerns: 
\bi
\item Missing related work, 
\item Details and motivation of the approach (e.g., the “Scale Up” approach), and
\item Details and justification of evaluation (e.g., does the benefit outweigh the cost). 
\ei
We hope the authors find the reviews useful in improving the manuscript and we look forward to the revision!}

Thank you very much for your comments. We have taken all the reviews into careful consideration and we have changed the manuscript to reflect those changes. We hope the new draft satisfies all the issues and concerns raised by the reviewers. 

To assist the reviewers in tracking all the changes we have incorporated in this version, we have ensured that we have prefixed all the recent additions with \respto{X-XX} to correspond to reviewers’ concerns.


\section*{Response to Reviewer 1}

Thank you very much for your detailed review. We have made several corrections, clarifications, and revisions as directed by your responses, we believe this new draft has improved thanks to your feedback. To assist in your review, we refer to specific locations of each of our changes using \respto{1-XX}.

\review{R1-1.~I am concerned with the “Scale-Up” approach. I understand that it could work very well most times. However, there will also be other cases where memory consumption constraints and I/O overhead trade-offs will be very different for workloads with original sizes, which will invalidate the Scale-Up heuristics.}



Theoretically, this is true. However, in this paper, we empirically show that such an effect is minimal. This a threat to validity. We have updated the threats to validity section (\tion{threats}) to highlight this \citeresp{1-1-B}. In particular, to minimize the threat, we choose a diverse set of workloads with different memory consumption and I/O overheads. Specifically:

\bi
\item
We note that the HiBench benchmarking suite offers a diverse set of workloads of various sizes, as shown in the following Table. 
We choose a range of workload sizes that fit within our available hardware (Intel(R) Xeon(R) E5-2660 CPU, 32GB memory, and 2TB of SSD storage). We summarize the various workload sizes below, and we highlight our choice in \colorbox{gray10}{gray}.

\begin{center}
\resizebox{0.22\textwidth}{!}{%
\begin{tabular}{V{1.5}l|l|lV{1.5}}
\hlineB{1.5}
Workload & Size & Studied \\ \hlineB{1.5}
tiny & 30KB & No \\ 
\rowcolor{gray10}small & 3MB & Yes \\ 
\rowcolor{gray10}large & 300MB & Yes \\ 
\rowcolor{gray10}huge & 3GB & Yes \\ 
gigantic & 30GB & No \\ 
bigdata & 300GB & No \\ \hlineB{1.5}
\end{tabular}%
}
\end{center}
Although the memory and I/O requirements for \texttt{small} and \texttt{huge} are different, our hardware can accommodate them. Further, we ignore the \texttt{tiny} workloads since the size (32kb) is too small to model the workload behavior accurately. 

\item We also pick a diverse set of workloads, \eg, \texttt{nutchindex} and \texttt{pagerank} are used in websearch; \texttt{svd} and \texttt{rf} are machine learning jobs; \texttt{sort} and \texttt{terasort} sort data; and finally \texttt{wordcount} operates on text data. These diverse job types ensure that the scale-out holds under different domains and under different workloads. 
\ei

In response to your question, we have also updated the experimental design section to highlight this~\citeresp{1-1-A}.


\review{R1-2. Can you explain how much manual effort is involved in pre-processing the configuration space (i.e., picking configurations and sub-samples)?}

Selecting the features during the pre-processing required a week’s worth of manual effort. We carefully examined the official documentation of Hadoop and Spark to enumerate all the configurable parameters. We discarded any static runtime parameters that should not be changed at runtime like paths, IP-address, hostnames, ssh-keys, etc. For the remaining configuration, we err on the side of caution. To make sure we cover all parameters related to runtime performance, we select all parameters that may impact the final performance. If we are not sure about a parameter, we include it in the sampling space.
Further, we referred to the review by Bonifacio~\etal~\cite{Bonifacio:research_review} on Hadoop which cites several studies and the parameters used by those studies. We compared our selected parameters with those of the previous paper to ensure that the chosen parameters are exhaustive.

Note that manual feature selection is a one-time effort undertaken at the beginning. We have updated the paper with additional text~\citeresp{1-2} to highlight this. 

\review{R1-3. How is your result sensitive to this manual process? If I put in a couple of more configurations, how does that affect the training/sampling performance and the result? For sub-sample during the pre-processing, are the final selected configurations limited to the sub-sampled configuration space? if so, isn’t there a trade-off there that worth evaluation --- the bigger configuration space will cause longer training time, but may produce better-performing configurations at the end?}


To answer your first question, ``If I put in a couple of more configurations, how does that affect the training/sampling performance and the result?’’, we note that during manual feature selection, we keep all the parameters except for static parameters such as those related to version (\eg, java\-.runtime\-.version),  file paths (\eg, hadoop\-.bin\-.path), authentication (\eg, hadoop\-.http\-.authentication\-.kerberos\-.keytab), server-address, and ID/names (\eg, mapreduce.output.basename). When in doubt, we include the parameter. This applies to both Hadoop and Spark. Therefore, we believe adding additional parameters will not adversely affect the performance. We have updated the current draft with the corresponding text in response to your comment~\citeresp{1-3}. 


As to your second question, ``For sub-sample during the pre-processing, are the final selected configurations limited to the sub-sampled configuration space? if so, isn’t there a trade-off there that worth evaluation --- the bigger configuration space will cause longer training time, but may produce better-performing configurations at the end?’’, we offer two answers: (1)~All parameters that may impact the performance have already been included as noted above, and (2)~In~\tab{sensitivity}, we list the 5 most influential parameters and we note that the performance gain offered by any additional parameters is marginal (less that 1\%). 

\review{R1-4. Why not use “tiny” workloads in scale-up experiments? Have you tried them?}

We ignore the \texttt{tiny} workloads since we discovered that their size (32kb) is too small to accurately model I/O, memory requirements, and run-time performances of for larger workloads such as \texttt{large} (300MB) and \texttt{huge} (3GB). We apologize for the missing description, we have now added this to our draft~\citeresp{1-4}.

\review{R1-5. The presentation of the MCMC algorithm is difficult to understand. For example, what exactly is the “distribution” and “target distribution”? And, why is the “acceptance/rejection” probability computed like that in equation 2?}

We apologize for the confusion here. We have added a new \S3 to better explain the theory behind EMCMC and why it is used~\citeresp{1-5}. Briefly, the key intuition behind MCMC is the observation that the configuration space is very large and we do not know before hand how to generate new configuration samples that offer better performance. To generate new configuration samples we need to know the probability distribution of the performance scores given a configuration. We refer to this distribution as the ``target distribution’’ and it is denote by $P(Y~|~c)$. We have added the definition and accompanying text in our new draft~\citeresp{1-5-A}.

We do not know the target probability distribution of the configurations. In such situations, MCMC based algorithms are well suited for generating new samples (configurations). There are many MCMC based algorithms, in this paper we make use of the Metropolis-Hastings algorithm (discussed in detail in the new \tion{mh}) since it works particularly well for high dimensional spaces such as in configuring big-data systems. 

Metropolis-Hastings algorithm uses a approximate probability distribution function (denoted by $Q(Y~|~c)$) in place of the unknown target probability distribution function ($P(Y~|~c)$).
At each step, the Metropolis-Hastings measures the \textit{Acceptance Probability} $A(c_{t+1}|c_{t})$ that determines if the new candidate ($c_{t+1}$) is accepted or rejected. The acceptance probability is determined by comparing the where the new candidate configuration ($c_{t+1}$) offers better performance than the old configuration (\ie, $Q(Y~|~c_{t+1}) > Q(Y~|~c_{t})$). The acceptance probability is given by:
\begin{equation*}
A(c_{t+1}|c_{t}) = min\left[1,\frac{Q(Y~|~c_{t+1})}{Q(Y~|~c_{t})}\right]
\end{equation*}

Based on the acceptance probability the new candidate configuration is accepted (in which case we use the candidate value in the next iteration) or rejected (in which case we discard the candidate value), and we reuse current value in the next iteration.

As to your question--- \textit{``why is the acceptance/rejection probability computed like that in equation 2?}’’, we note that it is a property of the Metropolis-Hastings algorithm. We compute it like so since it is used to determine whether we must keep a new configuration. The key component of the acceptance probability is that it is determined by the ratio $Q(Y~|~c_{t+1})/Q(Y~|~c_{t})$. If the new configuration $c_{t+1}$ is {\it more} likely to produce a better performance than the current configuration $c_t$ then $Q(Y~|~c_{t+1}) > Q(Y~|~c_t)$ and $Q(Y~|~c_{t+1})/Q(Y~|~c_{t}) > 1$. According to \eq{m}, $A(c_{t+1}|c_{t})=1$. and we will always accept the new configuration. 
If the new configuration $c_{t+1}$ is {\em less likely} to produce a better configuration than the current configuration, then $Q(Y~|~c_{t+1}) < Q(Y~|~c_t)$ and $Q(Y~|~c_{t+1})/Q(Y~|~c_{t}) < 1$. Here, $A(c_{t+1}|c_{t})$ is less than 1 and we will sometimes reject the new configuration. However, since the acceptance probability $A(c_{t+1}|c_{t})$ is non-zero, we may sometimes accept new configurations that perform worse than the previous configuration. The poorer the new configuration performs, the smaller the value of $A(c_{t+1}|c_{t})$ will be, making it less likely for us to accept a configuration with a bad performance scores. Using acceptance probability maintains the diversity among newly generated samples since it still keeps new samples dissimilar to the target distribution. We have added this our new draft~\citeresp{1-5-C}.


\review{R1-6. I understand that MMRE is not the most suitable metric in your context. However, I feel it would still be useful to know what it is for your algorithm and some alternative algorithms.?}

We apologize for the confusion here. MMRE is a measure of the predictive performance of an algorithm. We therefore calculate it as: 
\[
MMRE = \frac{|predicted-actual|}{actual} \cdot 100
\]
This applies only to machine learning algorithms that make some kind of prediction. Our approach does not offer a prediction per se, instead it performs an evolutionary search. Thus, we cannot measure the MMRE. We understand that this might be a source of confusion. We have therefore updated the evaluation section (\tion{eval}) by removing discussion on MMRE~\citeresp{1-6}.


\review{R1-7. Do we know the oracle results? Is there any way (e.g., within a small configuration space) that we can know the true-best configuration and then see how far away ConEx (and other techniques)’s results are from that true oracle performance?}

Unfortunately, we do not have access to the oracle results. We note that ConEx (and the underlying EMCMC algorithm) is most useful when the configuration space is large (such as with Hadoop and Spark) especially where the true optimum setting can be difficult, if not impossible, to find. In contrast with machine learning based methods of Nair \etal~\cite{nair2017faster} that attempt to predict for the best configuration, we use an evolutionary search based on MCMC to estimate the best configuration within a budget. If we have infinite budget, ConEX can theoretically converge on the true-best configuration. 

In response to your question, we have updated our text with the explanation~\citeresp{1-7}.

\review{R1-8. The discussion about “fifty production-scale jobs” is a little bit confusing. Where does this fifty come from? Are you saying the top 50’s performance are close to each other?}

We apologize for the confusion here. We have updated this section with better explanation~\citeresp{1-8}. Briefly, after running \tool, we identify the top 50 best performing configurations on a \texttt{small} workload. Next, during scale-up, we measure the performance gain offered by each of the top-1, top-3, top-10, and top-50 best configurations found on the \texttt{small} workload when used on the \texttt{large} and \texttt{huge} workloads. 

Our motivation arises from the observation that scale-up to larger workload sizes (which are 10$\times$ and 100$\times$ larger) may exhibit memory and performance constraints that small workload may not fully capture. 

We find that, in most cases, a configuration from among the top-50 best performing configurations found on a small workload produces a much higher performance gain than the top-1 configuration. We have included a new figure (see~\fig{scale_up} and \bareresp{1-8-B}). We have also added the corresponding text to explain this further in our draft~\citeresp{1-8-A}. 

As to your specific question of ``Where does this fifty come from?’’, we found that measuring the performance of over 50 configurations on \texttt{large} and \texttt{huge} workloads would incur a significant computational overhead with no further gain in performance (as shown in~\fig{scale_up} on page~\pageref{fig:scale_up}). 

Perhaps having to run 50 configurations on workloads of 3GB (large) and 30GB (huge) may incur much additional cost. This may be a potential trade-off that depends on the budget. If the budget available to the practitioners is very low, then just using the best configuration (\ie, Top-1) from the small workload may still produce notable improvements~(see~\tab{perf-improvement} in page~\pageref{tab:perf-improvement}). However, if an additional budget is available, practitioners may test the Top-3 to Top-50 configurations to find better overall improvements. Our new draft discusses this~\citeresp{1-8-C}. 

\review{R1-9.~Some previous work on configuration tuning for big data systems are not cited. Those work should be cited and discussed: “BestConfig: Tapping the Performance Potential of Systems via Automatic Configuration Tuning”, SOCC’17; “Datasize-aware high dimensional configurations auto-tuning of in-memory cluster computing”, ASPLOS’18; “A Probabilistic Graphical Model-based Approach for Minimizing Energy under Performance Constraints”, ASPLOS 2015.}

Thank you very much for pointing us to these papers. These works were not cited in our old draft, we have now updated our related work section to cite and discuss these papers~\citeresp{1-9-A}. Briefly we note that, there were subtle differences in the objectives, workload sizes, or jobs used in each of these papers compared to our work. Specifically, while some of these work used different tuning objectives (e.g., ASPLOS ‘15 used energy minimization as the aim) some other work use only a subset of the workloads and big-data systems used in our paper. Further, in several cases, we could not find an adequately documented replication package to reuse for comparison. 
That said, we note that sometimes, such as in BestConfig (from SOCC’17), we report much better performance gain for Hadoop (see Fig. 5 in BestConfig vs. Table 4 in our paper). 

In summary, we concur that this is a potential threat to validity and we have also updated our threats to validity section to highlight this issue~\citeresp{1-9-B}.


\section*{Response to Reviewer 2}

\review{(2.1) According to the last paragraph of Section 2.2, the limitation/challenges do not exist because the configuration space is too large. Why? Could you give a brief introduction here?}

We understand that this is potentially confusing. We intended to convey that limitations do not exist if the configuration space is \textit{too small}. When the configuration space is \textit{too large} (as with hadoop and spark), it exacerbates the limitation/challenges of ML based approaches. We have rewritten this paragraph to convey this better~\citeresp{2-1}.


\review{(2.2) Section 2.4 presents a novel Evolutionary-MCMC algorithm, which picks a random subset of the measured configurations without considering their measured performance (the original sentence is “We measure the performance of the initial configurations, and pick a random subset of the measured configurations”)? Please double check here.}

We apologize for the confusion here. This was a mistake on our part. We have fixed this sentence in our current draft~\citeresp{2-2}. 

\review{(2.3) the proposed EMCMC approach is general and can be applied to other problems? Could you please discuss its generality a bit?}

Thank you for pointing this out. EMCMC is a more general approach that can apply to several domains. The key premise of MCMC is that one does not have access to the probability distribution function from which to generate samples from. In such situations, MCMC proposes the use of a Markov Chain and an assumed probability distribution function to generate new samples. As the number of samples increases, the MCMC converges to the true probability distribution function. As noted in \tion{mcmc}, there are many MCMC algorithms such as Metropolis-Hastings, Hamiltonian Monte-Carlo, Reversible Jump, among other algorithms. 

Our paper uses an Evolutionary MCMC strategy as part of the CONEX framework to generate new samples. We can apply it to any domain where one needs not only to generate samples that belong to an unknown distribution but also requires the newly generated samples to exhibit some desired property (such as optimizing performance).
We have updated the related work section to highlight the general applicability of EMCMC~\citeresp{2-3}. 


\review{(2.4) Why 44 and 27 versions are taken as the stopping criteria, shown by Table 2?}

We apologize for the confusion here. 44 and 27 configurations are not the stopping criteria, rather they represent the total number of tunable configurations in hadoop and spark, respectively. As shown in Table 2, there are a total 901 configurations in hadoop and 212 in Spark. Not all of them impact the performance. Some configuration settings pertaining to runtime parameters such as paths, IP-address, hostnames, ssh-keys  cannot change during execution. So we discard them. For the remaining configurations, we err on the side of caution by making sure that we cover all parameters related to runtime performance; we select all parameters that somewhat impact the final performance. If we are not sure about a parameter, we include it in the sampling space. Further, we referred to the review by Bonifacio~\etal~\cite{Bonifacio:research_review} on Hadoop which cites several studies and the parameters used by those studies. We compared our selected parameters with those of the previous paper to ensure that the chosen parameters are exhaustive. This resulted in us keeping 44 configurations for Hadoop and 27 configurations for Spark. 

Note that this manual feature selection process took a week’s worth of investigation. It was, however, a onetime effort undertaken at the beginning. We have updated the paper with additional text~\citeresp{2-4} to highlight this. 


\review{(2.5) The proposed approach does not explore the whole space of each configuration parameter, but samples such space by defining small ranges of values of each parameter. Can you explain what influence does such sampling bring?}

The space of configuration options for each configuration parameter can be combinatorially large. Boolean configurations can take two options and configurations of categorical/string type can be assigned values from a few values. However, the number of options for integer and floating point configuration parameters is enormous. Therefore, we limit the search space to a range of values centered on the default parameter value. 

In theory, expanding the search space by increasing the number of values to sample may result in us finding a configuration that may produce a much larger performance gain. However, this may significantly increase the search time. We must account for this trade-off. To encourage further exploration, we make available a replication package (see \blue{\href{https://git.io/Jv958}{git.io/Jv958}}) where users may change these ranges of values as they see fit. In response to your question we have updated the threats to validity section to point this out~\citeresp{2-5}. 


We note the ranges of values for each parameter used in this paper was based on our best engineering judgement for the hardware we have run the workloads on. We find that the values of several of our the best parameters fall within of range defined by us. As an example, we summarize the \textit{best} value and our chosen range here--- {\blue{\url{http://tiny.cc/R2-5}}}. We see that in 70\% of the cases, we usually choose the best parameter values from within our range; in the remaining 30\% of the cases we found that the best parameter values were at the boundaries of our range (\ie, the values chosen were at the maximum or the minimum of the range we have defined.) 

\review{(2.6) Where is the CPU time of each Spark/Hadoop job? I guess Table 4(b) may be one of them?} 

Thank you for pointing this out. You are correct in that Table 4b (Table 5 in the new draft) highlights the CPU time of Hadoop. In the interest of space, we do not report the CPU times of Spark. However, we have made available a replication package with pre-configured docker containers for the Spark workloads to help measure the default runtimes and the performance gains. See~\blue{\href{https://git.io/Jv958}{git.io/Jv958}}. 

\review{(2.7) I am not sure whether the configuration selected is specific some job, general to all jobs in Hadoop/Spark. Maybe I ignore something in this paper? The usage scenario of the proposed approach is not clear to me.}

We apologize for the confusion here. To clarify, the configuration selected are specific to each of the jobs. We identify two usage scenarios.

In the first scenario, we consider a use case where a Big Data job is being deployed. Instead of profiling the big data job directly, one may deploy \tool on a small workload and get the best performing configurations and reuse that configuration for larger workloads (those which are 10$\times$ and 100$\times$ larger). As discussed in RQ1-2 we notice that best configurations found on a small workload can find better configurations for large workloads (with an average improvement of 20.50\%) and huge workloads (with an average improvement of 19.00\%). Note that we observe these improvements without having to run any large or huge workload. 

In the second scenario, we consider a use case where different jobs are being deployed on the big-data system, \eg, Hadoop is being used to deploy PageRank and WordCount as well. In such cases, instead of deploying \tool on each new task, one may reuse the best configurations identified by tool on a previous job (say PageRank) on the subsequent jobs. As shown in RQ1-4 we notice that other jobs can reuse best configurations found on a certain job. For instance, as tabulated in Table 6, if one were to use the best configuration found on TeraSort for WordCount, the performance improvement is 28.1\% (which is 6.6\% greater than the best configuration found using WordCount). Note again that we observe these improvements without having to run \tool on the new job. 

\section*{Response to Reviewer 3}
\review{(3.1) The notion of accepting/rejecting configurations is not very well explained. To make this part easier to follow for readers not familiar with the Metropolis-Hastings algorithm, it may help to provide an example, ideally one that uses configurations.}

We apologize for the confusion here. We created a new section (\S3) to better explain the theory behind EMCMC and its use case~\citeresp{3-1}. As per your advice, our new subsection (\S3.1) now details the Metropolis-Hastings algorithm from the perspective of optimizing configurations.

Briefly, we use MCMC based algorithms because the configuration space is very large and we do not know beforehand how to generate new configuration samples that offer better performance. To generate new configuration samples, we need to know the probability distribution of the performance scores given a configuration. We refer to this distribution as the ``target distribution’’ and it denote it by $P(Y~|~c)$.
MCMC based algorithms are well suited for generating new samples (configurations) in situations where the ``target distribution’’ $P(Y~|~c)$ is unknown. 

There are many MCMC based algorithms, in this paper we make use of the Metropolis-Hastings algorithm (discussed in the new \tion{mh}) since it works particularly well for high-dimensional spaces such as in configuring big-data systems. 

Metropolis-Hastings algorithm uses an approximate probability distribution function (denoted by $Q(Y~|~c)$) in place of the unknown target probability distribution function ($P(Y~|~c)$).
At each step, the Metropolis-Hastings measures the \textit{Acceptance Probability} $A(c_{t+1}|c_{t})$ that determines if the new candidate ($c_{t+1}$) is either accepted or rejected. The acceptance probability is determined by comparing the where the new candidate configuration ($c_{t+1}$) offers better performance than the old configuration (\ie, $Q(Y~|~c_{t+1}) > Q(Y~|~c_{t})$). The acceptance probability is given by:
\begin{equation*}
A(c_{t+1}|c_{t}) = min\left[1,\frac{Q(Y~|~c_{t+1})}{Q(Y~|~c_{t})}\right]
\end{equation*}

Based on the acceptance probability the new candidate configuration is accepted (in which case we use the candidate value in the next iteration) or rejected (in which case we discard the candidate value), and we reuse current value in the next iteration.


In response to your comment--- \textit{``The notion of accepting/rejecting configurations is not very well explained}’’, we have provided a better explanation~\citeresp{3-1-C}. We note that accepting/rejecting a sample (in our case a configuration) is a property of the Metropolis-Hastings algorithm and it computed because it is used to determine whether or not a new configuration must be kept. The key component of the acceptance probability is that it is determined by the ratio $Q(Y~|~c_{t+1})/Q(Y~|~c_{t})$. If the new configuration $c_{t+1}$ is {\it more} likely to produce a better performance than the current configuration $c_t$ then $Q(Y~|~c_{t+1}) > Q(Y~|~c_t)$ and $Q(Y~|~c_{t+1})/Q(Y~|~c_{t}) > 1$. According to \eq{m}, $A(c_{t+1}|c_{t})=1$. and we will always accept the the new configuration. 
If the new configuration $c_{t+1}$ is {\em less likely} to produce a better configuration than the current configuration, then $Q(Y~|~c_{t+1}) < Q(Y~|~c_t)$ and $Q(Y~|~c_{t+1})/Q(Y~|~c_{t}) < 1$. Here, $A(c_{t+1}|c_{t})$ is less than 1 and we will sometimes reject the new configuration. However, since the acceptance probability $A(c_{t+1}|c_{t})$ is non-zero, we may sometimes accept new configurations that perform worse than the previous configuration. The poorer the new configuration performs, the smaller the value of $A(c_{t+1}|c_{t})$ will be, making it less likely for us to accept a configuration with a bad performance scores. Using acceptance probability maintains the diversity among newly generated samples since it still keeps new samples dissimilar to the target distribution.


\review{(3.2) To sample the space of all syntactically configurations, the approach relies on some kind of configuration model, which defines valid and invalid configurations. The paper briefly refers to prior work on how this part works. I’d like to see a more detailed description of this part, along with a description of how much effort it is to construct this configuration model.}

We apologize for not providing enough details in our previous version as the checker is not a key contribution of this work, and we reused our previous work~\cite{tang2017interpreted}. We have now provided additional details on our configuration validity checker~\citeresp{3-2}. Briefly, we reuse an existing checker~\cite{tang2017interpreted}, our previous work, to formalize the configuration constraints in terms of COQ rules given to the prover~\cite{barras1997coq}. That tool provided templates to express these rules. We used the template along with the official documentation to write validation rules for both Hadoop and Spark. We note the templates make it easy to express the constraints; by expending a little effort on closely reading the documentation of the big-data systems we may update the template (with a full day worth of manual effort). To help further development, we make available these templates as part of our replication package (see \blue{\href{https://git.io/Jv958}{git.io/Jv958}}).


\review{(3.3) It isn’t clear how the configuration used to get some speedup was found. Under RQ1-2, the paper mentions that the authors evaluated each of the top-50 best performing configurations. Which of these configurations is used to compute Table 4, i.e., the evaluation of the scale-up and scale-out hypotheses?}

We apologize for the confusion here. To answer your question, ``which of these configurations is used to compute Table 4?’’, we note that to report the results, we used only the Top-1 (best) configuration obtained from the experiments run on small workloads. 

After running \tool, we identify the top 50 best performing configurations on a \texttt{small} workload. As per your recommendation, during scale-up, we measure the performance gain offered by each of the top-1, top-3, top-10, and top-50 best configurations found on the \texttt{small} workload when used on the \texttt{large} and \texttt{huge} workloads. 

Our motivation arises from the observation that scale-up to larger workload sizes (which are 10$\times$ and 100$\times$ larger in size) exhibit several memory and I/O constraints that are not fully represented by the small workload. Therefore, we wanted to explore if it was worth looking at configurations beyond Top-1.

We find that, in most cases, a configuration from among the top-50 best performing configurations found on a small workload produces a much higher performance gain than the top-1 configuration. We have included a new figure (see~\fig{scale_up} and \bareresp{3-2-B}) and corresponding text to explain this further in our draft~\citeresp{3-2-A}. 

\review{(3.4) Picking the best of the top-50 predicted configurations seems very unrealistic, because to find which of the top-50 is the best, one has to run all configurations, which imposes a huge cost.}

Thank you for pointing this out, this is a very good point. We agree with you that perhaps having to run 50 configurations on workloads of 3GB (large) and 30GB (huge) is intractable as it may incur much additional cost. We note that our report uses only Top-1 best configuration from a smaller workload to test the performance gains in the larger workloads. 

That said, this may be a potential trade-off and the choice to do so depends the budget. Our motivation in reporting the results of Top-50 configurations was to show the existence of the trade-off between the budget and the performance. Specifically, better performance gains may be achieved by evaluating up to top-50. If no budget is available, then just using the best configuration (\ie, Top-1) from the small workload may still produce notable improvements~(see~\tab{perf-improvement} in page~\pageref{tab:perf-improvement}). Using Top-1 would require no additional measurements on larger workloads. However, if additional budget is available, practitioners may evaluate the Top-3 to Top-50 configurations to find better overall improvements. Our new draft discusses this~\citeresp{3-4}. We note that using any more than the top-50 configurations does not offer any notable gains in performance as shown in Figure 5. 

\balance

\review{(3.5) On p11 (first paragraph), the authors briefly describe that picking among the top candidates doesn’t make much of a difference, but the detailed results are omitted. Is this true for top-3, top-5, or top-50? Please provide more detailed results.}

We apologize for the misleading text in that paragraph. We intended to state that picking any configuration from among the top 50 configurations offers significant improvements over the default (see Figure 5). However, we note that exploring the top 50 configurations instead of just picking the top-1 may be more beneficial since larger workload sizes (which are 10$\times$ and 100$\times$ larger) exhibit several memory and I/O constraints that may not be fully represented by the top-1 configuration of the small workload. 

We found that, in most cases, a configuration from among the top-50 best performing configurations found on a small workload did produce a much higher performance gain than just using the top-1 configuration. We have included a new figure (see~\fig{scale_up} and \bareresp{3-2-B}) and corresponding text to explain this further in our draft~\citeresp{3-2-A}. 


\review{(3.6) Assuming that the authors picked the best of the top-50 configurations, I’d be more interested in a setup where only the top-1 suggestion is used. This seems more realistic, as it doesn’t require running all top-50 configurations.}

Thanks for highlighting this. Our results (current Table 4) reports the Top-1. We apologize for the lack of clearity in our old draft. Our new draft clarifies this~\citeresp{3-6}. We have now included a new figure (Figure 5) to show the difference between Top-1 to Top-50 best configurations. 

\review{(3.8) To what extent is the proposed solution specific to big-data jobs? The general idea of addressing a search problem through a combination of genetic search and MCMC sampling seems much more general. The paper could become relevant beyond its current scope by further discussing the generality of the proposed algorithm.}

Thank you for pointing this out. EMCMC is a more general approach that can apply to several domains. The key premise of MCMC is that one does not have access to the probability distribution function from which to generate samples from. In such situations, MCMC proposes the use of a Markov Chain and an assumed probability distribution function to generate new samples. As the number of samples increases, the MCMC converges to the true probability distribution function. As noted in \tion{mcmc}, there are many algorithms that can be used for MCMC such as Metropolis-Hastings, Hamiltonian Monte-Carlo, Reversible Jump, among other algorithms. 

Our paper uses an Evolutionary MCMC strategy as part of the CONEX framework to generate new samples. We can apply it to any domain where one needs not only to generate samples that belong to an unknown distribution but also requires the newly generated samples to exhibit some desired property (such as optimizing performance).
We have updated the related work section to highlight the general applicability of EMCMC~\citeresp{3-8}. 


\balance

\review{(3.9) Section 4.4 says “these accuracy measures are best suited for traditional machine learning based performance optimization models”. Why is this?}

We apologize for the confusion here. In our old text, ``these accuracy measures’’ referred to MMRE which is a measure of the predictive performance of a Machine learning algorithm. We therefore calculate it as: 
\[
MMRE = \frac{|predicted-actual|}{actual} \cdot 100
\]
This applies only to machine learning algorithms that make some kind of prediction. Our approach does not offer a prediction per se, instead it performs an evolutionary search. Thus, we cannot measure the MMRE. We understand that this might be a source of confusion. We have therefore updated the evaluation section (\tion{eval}) by removing discussion on MMRE~\citeresp{3-9}.


\review{(3.10) The paper says that it ``directly used the model published by Nair et al.’’. The prior work seems to have used a different benchmark, which means reusing a pre-trained model isn’t meaningful. Did the authors train the Nair et al. model on data from the benchmarks used in this submission?}

Thanks for highlighting this. The text in our old draft was misleading. By ``directly used the model’’ we meant that we re-used the machine learning model but for the rest we replicated the exact experimental method proposed by Nair \etal We used the replication package provided by Nair \etal (available at \href{https://github.com/ai-se/Reimplement/tree/cleaned\_version}{https://github.com/ai-se/Reimplement/tree/cleaned\_version}) as a reference for our implementation. 
We have now fixed this sentence in our paper~\citeresp{3-10}.
